# Supplementary material for: Resolution dependence of most probable pathways with state-dependent diffusivity
Source: arXiv:2402.01559 ancillary file (2024-02-02)
Supplement: Supplementary file 1 [file supplement.pdf]

# Resolution dependence of most probable pathways with state-dependent diffusivity – Supplemental Material –

Alice L. Thorneywork,[1,2] Jannes Gladrow,[3] Ulrich F. Keyser,[2] Michael E. Cates,[4] Ronojoy Adhikari,[4] and Julian Kappler[4,5]

[1] *Physical and Theoretical Chemistry Laboratory, University of Oxford, South Parks Rd, Oxford OX1 3QZ, United Kingdom*
[2] *Cavendish Laboratory, University of Cambridge, J J Thomson Ave, Cambridge CB3 0HE, United Kingdom*
[3] *Microsoft Research, Station Rd, Cambridge CB1 2FB, United Kingdom*
[4] *Department of Applied Mathematics and Theoretical Physics, Centre for Mathematical Sciences, University of Cambridge, Wilberforce Rd, Cambridge CB3 0WA, United Kingdom*
[5] *Arnold Sommerfeld Center for Theoretical Physics (ASC), Department of Physics, Ludwig-Maximilians Universität München, Theresienstraße 37, D-80333 Munich, Germany*

(Dated: February 2, 2024)

## S1. PARAMETRIZATION OF LANGEVIN EQUATION

To parametrize the Itô Eq. (5) from experimental time series, we use the approach described in Ref. [1], which is based on the Kramers-Moyal coefficients

$$\frac{\langle \Delta X_{\Delta t^*} \rangle|_{X_0=x}}{\Delta t^*} = a(x) + \mathcal{O}(\Delta t^*), \quad \text{(S1)}$$

$$\frac{\langle \Delta X^2_{\Delta t^*} \rangle|_{X_0=x}}{\Delta t^*} = 2D(x) + \mathcal{O}(\Delta t^*), \quad \text{(S2)}$$

where $\Delta X_{\Delta t^*} \equiv X_{\Delta t^*} - X_0$ is the increment during the lag time $\Delta t^*$, and where the averages on the left-hand side are over all realizations of the Langevin Eq. (5) with initial condition $X_0 = x$.

To evaluate the left-hand side of Eqs. (S1), (S2) using experimental time series, we bin space using a bin width $\Delta x = 0.05\,\mu$m with bin centers $\hat{x}_i$. For bin center $\hat{x}_i$ we estimate the $k$-th moment as

$$\langle \Delta X^k_{\Delta t^*} \rangle|_{X_0=\hat{x}_i} \approx \frac{1}{N_i} \sum_\alpha (X_{\alpha+l} - X_\alpha)^k, \quad \text{(S3)}$$

where the sum on the right-hand side is over all the $N_i$ recorded trajectory increments for which $X_\alpha \in [\hat{x}_i - \Delta x/2, \hat{x}_i + \Delta x/2]$, and where $l = \Delta t^*/\Delta t$ with $\Delta t$ the time step of the recorded time series.

Substituting Eq. (S3) into Eqs. (S1), (S2), and neglecting the terms of order at least $\Delta t^*$ on the right-hand side of the equations, we obtain

$$a(\hat{x}_i) = \frac{1}{\Delta t^* N_i} \sum_\alpha (X_{\alpha+l} - X_\alpha), \quad \text{(S4)}$$

$$D(\hat{x}_i) = \frac{1}{2\Delta t^* N_i} \sum_\alpha (X_{\alpha+l} - X_\alpha)^2. \quad \text{(S5)}$$

To estimate the drift and diffusivity profile, we evaluate the right-hand side of Eqs. (S4), (S5) using our experimental time series.

The lag time $\Delta t^*$, which is a multiple of the time step $\Delta t$ of the time series, should be so small that it is acceptable to neglect the $\mathcal{O}(\Delta t^*)$ terms in Eqs. (S1), (S2). On the other hand, the lag time $\Delta t^*$ should be so large that i) the dynamics of the colloidal particle is approximately described by the Itô Eq. (5) (meaning that non-Markovian or inertial effects are negligible), and that ii) measurement errors can be neglected. As discussed in Ref. [1], for the length scales of the channel and colloidal particle considered here, hydrodynamic effects are negligible on the millisecond time-scale dynamics we probe; furthermore, the error in the particle tracking becomes smaller than the typical particle displacement for times $\Delta t^* \gtrsim 10\,$ms. We therefore evaluate Eqs. (S4), (S5) for the three lag times $\Delta t^* = 20, 30, 40\,$ms, and show the resulting diffusivity and drift profiles in Fig. S1 (a), (b).

As the figure shows, both the inferred drift and diffusivity profiles are identical for all three lag times $\Delta t^*$ considered (except for some minor deviations in the diffusivity profile for $\Delta t^* = 20\,$ms, which are most prominent for $x \approx 0\,\mu$m). The independence of the drift and diffusivity on the lag time shows that for $\Delta t^* = 30\,$ms, the dynamics of the colloidal particle is well-described by the Itô Eq. (5); for all analytical calculations in the main text we therefore use the inferred drift and diffusivity profile for $\Delta t^* = 30\,$ms.

To evaluate analytical formulas on the parametrized drift and diffusivity, we smooth the inferred profiles using a Hann window of width $1.5\,\mu$m (Fig. 1 features a comparison of the directly inferred and smoothed versions), and construct cubic spline interpolation functions from the smoothed curves.

## S2. STEADY STATE

The exit rates we calculate theoretically only require knowledge about the diffusivity $D$ and the drift $a$. It is instructive to also consider the potential $U$ obtained from the steady-state distribution $P_{\rm ss}$ within the corrugated

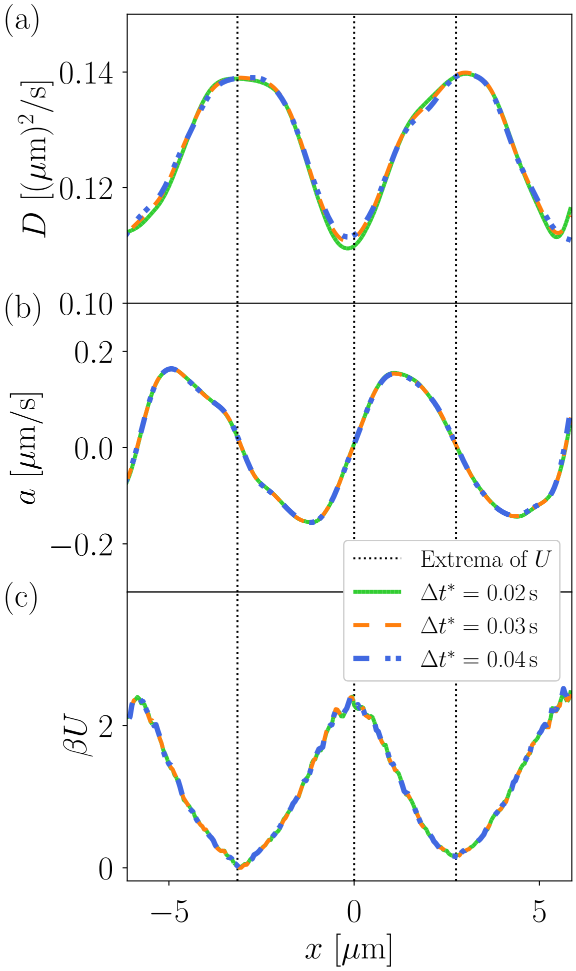


Figure S1. (a) Diffusivity and (b) drift profiles obtained from evaluating Eqs. (S4), (S5) on recorded experimental time series for the lag times $\Delta t^* = 20\,\mathrm{ms}$ (green solid lines), $\Delta t^* = 30\,\mathrm{ms}$ (orange dashed lines), and $\Delta t^* = 40\,\mathrm{ms}$ (blue dash-dotted lines). The drift and diffusivity profiles are smoothed using a Hann window of width $1.5\,\mu\mathrm{m}$. (c) Potential landscape obtained from evaluating Eq. (S8) using the inferred drift and diffusivity profiles, as shown in subplot (a), (b). While subplots (a), (b) show smoothed versions of drift and diffusivity, for the evaluation of Eq. (S8) and subplot (c) we use the non-smoothed versions. All potential landscapes are shifted in the $y$-axis, so that their lowest local minimum is at value $U = 0$. The vertical dashed lines in subplots (a), (b), (c) denote the local extrema of the potential landscape for $\Delta t^* = 30\,\mathrm{ms}$ (orange dashed line in subplot (c)). The legend refers to all subplots.

channel via Boltzmann inversion,

$$\beta U(x) = -\ln\left(L P_{\mathrm{ss}}(x)\right), \tag{S6}$$

where $L$ is an arbitrary length scale to make the argument of the logarithm dimensionless.

The corrugated channel we consider in our experiments is coupled to bulk fluid reservoirs on both ends. Our physical system thus effectively has absorbing boundary conditions, which implies a steady-state density that vanishes everywhere inside the channel.

To obtain a nontrivial steady-state distribution within the channel, we therefore use the inferred drift and diffusivity to calculate the reflecting-boundary steady state, which follows from Eq. (5) as [2]

$$P_{\mathrm{ss}}(x) = \frac{\mathcal{N}(x_0)}{D(x)} \exp\left[\int_{x_0}^{x} \mathrm{d}x' \, \frac{a(x')}{D(x')}\right]. \tag{S7}$$

where $x_0$ is an arbitrary reference point and $\mathcal{N}(x_0)$ is a constant that ensures proper normalization of the distribution.

Upon substituting Eq. (S7) into Eq. (S6), we obtain

$$\beta U(x) = \ln\left[\frac{D(x)}{D_0}\right] - \int_{x_0}^{x} \mathrm{d}x' \, \frac{a(x')}{D(x')} + U_0, \tag{S8}$$

where $D_0$ is an arbitrary diffusivity scale and $U_0 = -\ln[L D_0 \mathcal{N}(x_0)]$ is independent of $x$.

Using the inferred drift and diffusivity profiles for $\Delta t^* = 20, 30, 40\,\mathrm{ms}$, as described in Sect. S1, we evaluate Eq. (S8). We shift each potential so that the lowest local minimum is at value $U = 0$ . We show the resulting three potentials in Fig. S1 (c), all of which agree very well with each other. In particular, all potentials clearly show two local minima, at $x_{\mathrm{left}} \approx -3.2\,\mu$m and $x_{\mathrm{right}} \approx 2.8\,\mu$m, separated by a barrier with maximum at $x_{\mathrm{top}} = 0$ (vertical dashed lines).

## S3. CLONING ALGORITHM FOR MEASURING SOJOURN PROBABILITIES AND EXIT RATES

To estimate the sojourn probability for radius $R$ and path $\varphi$ from measured time series we use the cloning algorithm described in Ref. [1] and implemented in Ref. [3], which we now briefly summarize.

In short, the key idea of the algorithm is to estimate the sojourn probability by considering random samples of recorded trajectories, discarding each trajectory once it first leaves the instantaneous tube $[\varphi(t) - R, \varphi(t) + R]$, and using the fraction of surviving trajectories as an estimate for the sojourn probability. To overcome the exponential decay of sample trajectories that have never left the tube, we at evenly spaced time intervals infer the probability distribution of surviving trajectories within the instantaneous tube domain, and draw new random samples of recorded trajectories according to this distribution [1].

More explicitly, for a short duration $t \in [0, \Delta\mathcal{T}]$, we follow a number $M_0$ of randomly selected recorded trajectory snippets that start close to the initial position of $\varphi$. We discard each trajectory once it leaves the instantaneous tube domain $[\varphi(t) - R, \varphi(t) + R]$ for the first time, and denote the number of remaining trajectories at time $t_j = j \cdot \Delta t$ by $M_{0,j}$. For $t_j \in [0, \Delta\mathcal{T}]$, we then estimate the sojourn probability as

$$P_R^{\varphi}(t_j) = \frac{M_{0,j}}{M_0}. \tag{S9}$$

At time $\Delta\mathcal{T} = J \cdot \Delta t$, we create a histogram of the final positions of all the sample trajectories that have never left the tube; for this histogram we use a bin width $\Delta x = 0.05\,\mu$m.

To estimate the sojourn probability for the time interval $[\Delta\mathcal{T}, 2\Delta\mathcal{T}]$, we randomly sample $M_1$ snippets of recorded trajectories with probabilities according to the histogram of final positions from the time interval $[0, \Delta\mathcal{T}]$. We then follow those trajectories, and again discard each trajectory once it exits the domain $[\varphi(t) - R, \varphi(t) + R]$ for the first time, to obtain the sojourn probability in the time interval $[\Delta\mathcal{T}, 2\Delta\mathcal{T}]$ as

$$P_R^{\varphi}(\Delta\mathcal{T} + j\Delta t) = \frac{M_{0,J}}{M_0}\frac{M_{1,j}}{M_1}, \quad \text{(S10)}$$

where $M_{1,j}/M_1$ is the fraction of the newly drawn trajectories that have never left the tube until time $t = \Delta\mathcal{T} + j\Delta t$.

To obtain the sojourn probability until time $t_f$, we iteratively repeat this procedure until $K \cdot \Delta\mathcal{T} = t_f$.

From the sojourn probability, we calculate the exit rate via the relation $\alpha_R^{\varphi} = -\dot{P}_R^{\varphi}/P_R^{\varphi}$, where we use the central difference scheme to evaluate the time derivative numerically.

Unless explicitly stated otherwise, at iteration step $k \geq 1$ we use a variation of the estimation formula from Ref. [1] to choose the number of drawn trajectories $M_k$. The basic idea is to estimate the decay of the sojourn probability during the next iteration from the recent behavior of the exit rate, and to choose $M_k$ so that we obtain approximately a given number of remaining trajectories at the end of the next iteration. More explicitly, we fit a function $\hat{\alpha}_{\text{lin}}(t) = p_1(t - k\Delta\mathcal{T}) + p_2$ to the last 0.8 s of measured exit rate and set $\alpha_{\text{lin}}(t) = \max\{p_1, 0\}(t - k\Delta\mathcal{T}) + p_2$. Using $\max\{p_1, 0\}$ instead of $p_1$ means we consider a constant exit rate $\alpha_{\text{lin}} \equiv p_2$ if the exit rate is expected to decrease during the next iteration (this replacement ensures that the estimated number of trajectories, Eq. (S11) below, does not decrease too fast during periods of time where the exit rate decreases rapidly). We use the function $\alpha_{\text{lin}}$ to estimate the remaining trajectories at the end of the next iteration as

$$M_{k,\text{final}} = M_k \exp\left[-\int_{k\Delta\mathcal{T}}^{(k+1)\Delta\mathcal{T}} dt\, \alpha_{\text{lin}}(t)\right]. \quad \text{(S11)}$$

Evaluating the temporal integral in the exponent and solving the equation for $M_k$, we obtain

$$M_k = M_{k,\text{final}} \exp\left(\max\{p_1, 0\}\Delta\mathcal{T}^2 + p_2\Delta\mathcal{T}\right). \quad \text{(S12)}$$

We use this formula to choose $M_k$, and use $M_{k,\text{final}} = 10^5$ unless noted otherwise.

For all results shown in this paper, we use $\Delta\mathcal{T} = 0.25$ s and $\Delta x = 0.05\,\mu$m; in Ref. [1] it is shown that these parameters are adequate for the typical diffusivity, drift, and trajectory speeds considered in the present system.

## S4. ALGORITHM FOR DETERMINING MOST PROBABLE TUBE CENTERS/MOST PROBABLE PATHS

To calculate most probable tubes (MPTs) we employ the following algorithm used in Ref. [1]. For this, we approximate the space of paths with boundary conditions $\varphi(0) = x_{\text{left}}$, $\varphi(t_f) = x_{\text{right}}$, by the parametrization

$$\varphi(t) = x_{\text{left}} + (x_{\text{right}} - x_{\text{left}})\frac{t}{t_f} + \sum_{n=1}^{N}\frac{c_n}{n^2}\sin\left(n\pi\frac{t}{t_f}\right), \quad \text{(S13)}$$

so that a path is represented by an $N$-dimensional vector $\vec{c} = (c_1, ..., c_N)$; note that for any vector $\vec{c} \in \mathbb{R}^N$, the path Eq. (S13) fulfills the boundary conditions $\varphi(0) = x_{\text{left}}$, $\varphi(t_f) = x_{\text{right}}$. Obtaining the MPT center then means minimizing the $N$-dimensional function $P_R(\vec{c}) \equiv P_R^{\varphi}(t_f)$, where $P_R^{\varphi}$ is the sojourn probability along the path $\varphi$ defined by Eq. (S13).

We calculate the MPT center both using sojourn probabilities directly measured from the experimental data as described in Sect. S3, and by evaluating the theoretical sojourn probability on the parametrized Langevin dynamics from Sect. S1. In both cases, we use a cma-es minimization algorithm [4] with initial condition $\vec{c} = (0, ..., 0)$ and a diagonal initial variance $\sigma_{\text{cma}} = 0.5$.

To evaluate $P(\vec{c})$ using experimental data, we use the cloning algorithm from Sect. S3. We use $N = 20$ modes in Eq. (S13), $M_0 = 10^4$, and $M_{k,\text{final}} = 2000$ for $k \geq 1$. Since, for a finite number of samples $M_k$, the inferred sojourn probability is a random variable, we run 5 independent minimizations for each radius $R$, resulting in 5 candidates for the MPT center. For each of the 5 candidates, we evaluate the sojourn probability using $M_0 = 10^5$, $M_{k,\text{final}} = 10^5$, and use as MPT center the path with the largest sojourn probability.

To evaluate $P(\vec{a})$ theoretically, we use Eqs. (1), (2) together with the perturbative expression Eq. (6) to order $R^0$ (inclusive). Unless stated otherwise, we for the theoretical evaluation use $N = 40$ modes in the parametrization Eq. (S13). We remark that the python module PyTubular [5] (which implements the analytical exit rate Eq. (6)), comes with an example notebook that implements this minimization procedure for a given drift and diffusivity profile.

## S5. COMPARISON OF EXIT RATE TO ORDER $R^0$ AND $R^2$

In Eq. (6) we consider the tubular exit rate to order $R^0$. We now show that this order is sufficient for all the scenarios considered in the main text. We achieve this by demonstrating that incorporating the next-order term does not change any of the results significantly. For this

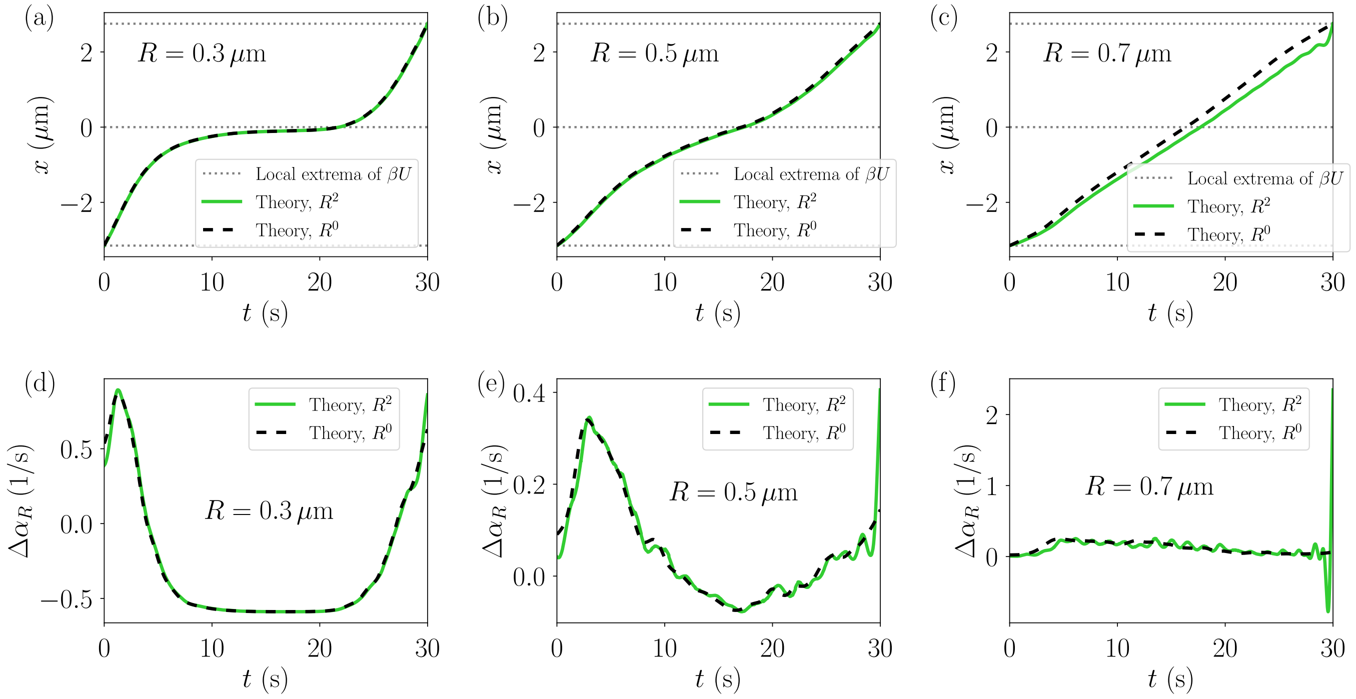


Figure S2. (a), (b), (c): The solid and dashed lines show the most probable tube center Eq. (3) evaluated using the perturbative exit rate to order $R^0$ (Eq. (6), black dashed lines) and to order $R^2$ (Eq. (S14), green solid lines). We present results for radius (a) $R = 0.3\,\mu$m, (b) $R = 0.5\,\mu$m, and (c) $R = 0.7\,\mu$m. To minimize the respective functional, we use the path parametrization from Sect. S4, and evaluate the exit rate along each path using the diffusivity and drift profile corresponding to Fig. 1 (b), (c). The horizontal dotted lines denote the local extrema of the potential $\beta U$ from Fig. 1 (c). (d), (e), (f) show the exit-rate difference Eq. (4) for the paths from subplots (a), (b), (c). The curves are evaluated using the corresponding perturbative exit rate (Eq. (6) for the order $R^0$ theory, shown as black dashed lines; Eq. (6) for the order $R^2$ theory, shown as green solid lines). The subplots show results for (d) $R = 0.3\,\mu$m, (e) $R = 0.5\,\mu$m, (f) $R = 0.7\,\mu$m. For all theoretical evaluations of exit rates we use the diffusivity and drift profile corresponding to Fig. 1 (b), (c). Note that the order-$R^0$ results in subplots (a-c), and (d-f) are replots of the corresponding curves from Figs. 1, 2.

we consider the exit rate to order $R^2$,

$$\alpha_R^{\varphi}(t) = \frac{\alpha_{\text{free}}^{\varphi}(t)}{R^2} + \alpha^{\varphi,(0)}(t) + \alpha^{\varphi,(2)} R^2 + \mathcal{O}(R^4), \quad \text{(S14)}$$

where $\alpha_{\text{free}}^{\varphi}$ and $\alpha^{\varphi,(0)}$ are given by Eqs. (7), (8), and the explicit expression for $\alpha^{\varphi,(2)}$ is given in the accompanying paper Ref. [6] (note that in the reference time-dependent tube radii are considered; therefore, what we denote by $R$ here is denoted by the symbol $R_0$ in the reference).

In Figs. 1, 2, we showed results for the MPT and the corresponding exit-rate difference for $R = 0.3\,\mu$m, $R = 0.5\,\mu$m, $R = 0.7\,\mu$m. For each of these radii, we determine the theoretical MPT using the exit rate to order $R^2$, Eq. (S14). In Fig. S2 we compare the resulting MPTs and exit-rate differences to the order-$R^0$ results. From the figure we see that the results theoretical results to order $R^0$ and $R^2$ agree very well, with some minor deviations starting to appear for the largest radius considered $R = 0.7\,\mu$m (most prominently in Fig. S2 (c)). Overall, from Fig. S2 we conclude that for the MPT centers and exit rates considered in the main text, the theoretical exit rate to order including $R^0$ is sufficient.

## S6. THEORETICAL ESTIMATE FOR THE CROSSOVER FROM DIFFUSIVITY-DOMINATED MPT TO LAGRANGIAN-DOMINATED MPT

In Fig. 1 of the main text we observed that the MPT for a barrier crossing changes qualitatively as a function of the radius. While for small radius the MPT lingers at the maximum, the MPT crosses the maximum without slowing down noticeably as the radius is increased. We now estimate the crossover radius at which the MPT switches between lingering and crossing without slowing down significantly.

For this we consider two paths, resting at $x_{\text{top}}$ and $x_{\text{left}}$ respectively, with corresponding exit rates $\alpha_R^{x_{\text{top}}}$, $\alpha_R^{x_{\text{left}}}$. At small enough radius we expect $\alpha_R^{x_{\text{top}}} < \alpha_R^{x_{\text{left}}}$, as then Eq. (7) dominates the exit rate, and we have $D(x_{\text{top}}) < D(x_{\text{left}})$. At some larger radius we expect $\alpha_R^{x_{\text{top}}} > \alpha_R^{x_{\text{left}}}$, due to the confinement of the potential well around $x_{\text{left}}$ and the potential energy instability at the barrier top $x_{\text{top}}$ (as described by the term $\partial_x a$ in Eq. (8)).

As a proxy for the radius at which Eq. (6) switches over from low-diffusivity-preferring MPT to Lagrangian-

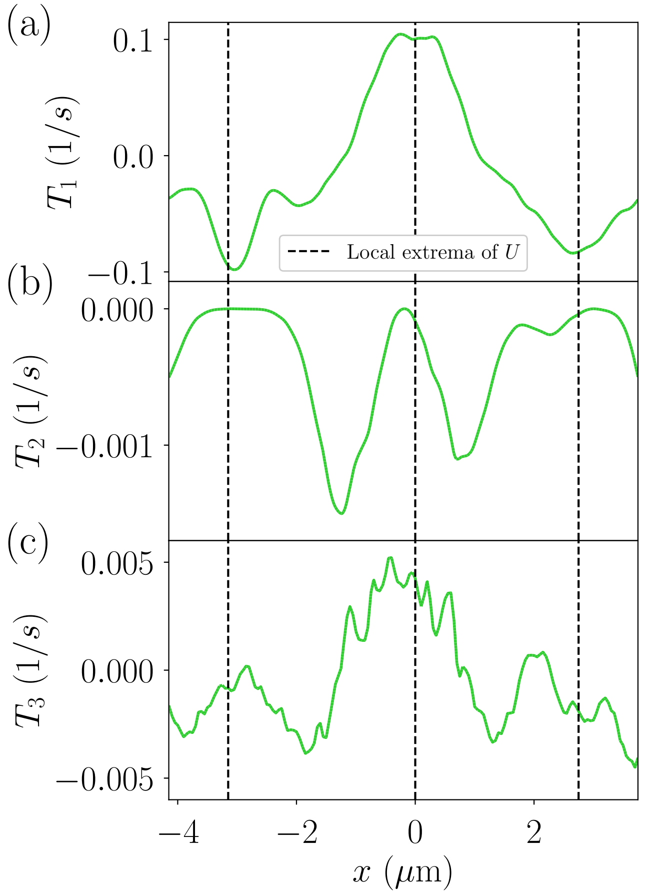


Figure S3. The subplots show the three terms (a) Eq. (S16), (b) Eq. (S17), (c) Eq. (S18), which contribute to the Lagrangian Eq. (8). For evaluations of $a$, $D$ we use the smoothed diffusivity and drift shown in Fig. S1. We show the local extrema of the potential as vertical dashed lines.

dominated MPT, we use the radius $R_c^{\text{theory}}$ defined by

$$\alpha^{x_{\text{top}}}_{R_c^{\text{theory}}} = \alpha^{x_{\text{left}}}_{R_c^{\text{theory}}}. \tag{S15}$$

Since the constant paths at $x_{\text{left}}$ and $x_{\text{right}}$ have vanishing velocity and are close to potential energy extrema, the term $\dot{\varphi} - a$ is small and we neglect the corresponding terms in Eq. (8). We show the remaining terms,

$$T_1 \equiv \frac{1}{2}\partial_x a, \tag{S16}$$

$$T_2 \equiv -\frac{1}{16}\left(\pi^2 - 3\right)\frac{(\partial_x D)^2}{D}, \tag{S17}$$

$$T_3 \equiv \frac{1}{4}\left(\frac{\pi^2}{6} - 1\right)\partial_x^2 D, \tag{S18}$$

as a function of $x$ in Fig. S3. We observe that $|T_1|$ is typically at least one order of magnitude larger than $|T_2|$, $|T_3|$, meaning for our system the effects on the exit rate due to the derivatives of $D$ are negligible as compared to the effects due to the drift $a$. We hence approximate

$$\alpha_R^x \approx \frac{\pi^2 D(x)}{4R^2} + \frac{1}{2}(\partial_x a)(x) \tag{S19}$$

for a constant path resting at a point $x$.

Substituting Eq. (S19) in Eq. (S15) and solving for $R_c^{\text{theory}}$, we obtain the theoretical crossover radius

$$R_c^{\text{theory}} = \pi\sqrt{-\Delta D/[2\Delta(\partial_x a)]} \approx 0.59\,\mu\text{m}, \tag{S20}$$

where $\Delta D \equiv D(x_{\text{left}}) - D(x_{\text{top}})$, $\Delta(\partial_x a) \equiv (\partial_x a)(x_{\text{left}}) - (\partial_x a)(x_{\text{top}})$.

Our theoretical estimate $R_c^{\text{theory}} \approx 0.59\,\mu\text{m}$ is 34% larger than the numerical $R_c \approx 0.44\,\mu m$ based on the full theoretical exit rate to order $R^0$ (c.f. Fig. 3). We rationalize the deviation between theoretical estimate and numerical crossover radius by the approximations made in calculating the former; in particular, $R_c^{\text{theory}}$ neglects that, due to the boundary conditions, the barrier-crossing MPT does not rest at the barrier top the whole path duration.

## S7. MOST PROBABLE TUBE CENTERS FOR SMALLER RADII

The smallest tube radius for which we consider the MPT in the main text is $R = 0.3\,\mu\text{m}$, c.f. Fig. 1 (d). Due to the finite temporal and spatial resolution of our experimental data, it is not possible to use the algorithm from Sect. S3 to infer the exit rate for arbitrary small radius. There is of course no small-radius limitations for evaluating the theoretical exit rate on a parametrized diffusivity and drift profile (although at sufficiently small length- and timescale, the overdamped Langevin model is expected to break down so that the $R \to 0$ limit of the parametrized model is not the $R \to 0$ limit of the physical colloidal particle, for which at some point inertial effects will become relevant).

To further demonstrate that for asymptotically small tube radius the MPT aims to minimize the diffusivity, we now consider the theoretical MPTs for some small values of the tube radius. In Fig. S4 we show a replot of the theoretical MPT for $R = 0.3\,\mu\text{m}$ from Fig. 1 (d), together with theoretical MPT for $R = 0.1\,\mu\text{m}$ and $R = 0.05\,\mu\text{m}$. The figure shows that as the radius is decreased, the MPT moves towards the minimum of the diffusivity more quickly and remains there longer. This is because for decreasing radius the free-diffusion term in Eq. (6) is more dominant; this term is proportional to the diffusivity, and so the MPT seeks to spend time at the position where the diffusivity is minimized. From Fig. S4 and the form of Eq. (6) for asymptotically small radius it is apparent that in the asymptotic limit of vanishing radius, the most probable path will almost instantaneously move to the minimum of the diffusivity, and remain there practically until the final time.

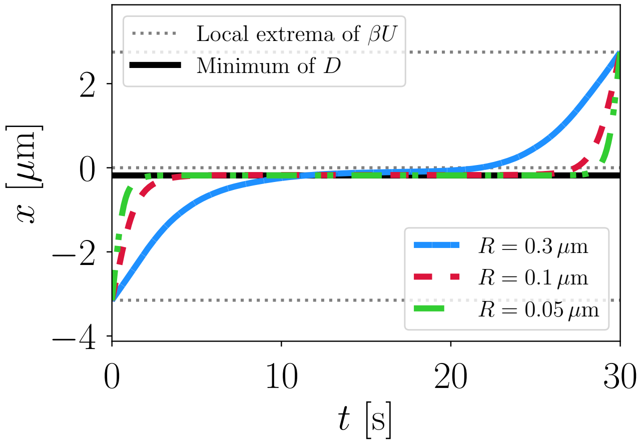


Figure S4. The colored solid and broken lines denote the most probable tube for a path that starts at $x_{\mathrm{left}}$ and ends at $x_{\mathrm{right}}$ after a duration $T = 30\,s$. For each radius, we obtain the most probable tube by minimizing Eq. (3), using the theoretical exit rate Eq. (6) to order $R^0$ (inclusive), as well as the algorithm presented in Sect. S4. While for $R = 0.3\,\mu$m we use $N = 40$ modes to parametrize the space of paths, for $R = 0.05\,\mu$m and $R = 0.1\,\mu$m we use $N = 80$ modes to better resolve the fast motion at the initial and final times of the respective trajectory.

## S8. EXIT RATES VS. EXIT RATE DIFFERENCES

In the main text and throughout this supplemental material we work with exit rate differences as defined in Eq. (4). In this section we discuss the advantage of considering exit-rate differences, as compared to absolute exit rates. For this, we consider the paths $\varphi^*$, $\psi$ from Fig. 1 (d)-(f), and compare the experimental exit rates along either path to the theoretical result Eq. (6).

For radius $R = 0.3\,\mu$m (left column), $R = 0.5\,\mu$m (center column), $R = 0.7\,\mu$m (right column), we show the experimental exit rate along the MPT center $\varphi^*$ in the first row of Fig. S5. In the second row we plot the exit rate along the constant path $\psi$, and in the third row the corresponding exit-rate difference.

All green curves in Fig. S5 are obtained from our experimental time series via the cloning algorithm described in App. S3, using the experimental time series at full temporal resolution $\Delta t = 0.002\,$s. This is precisely the algorithm parameters used in the main text, and consequently the green curves in subplots (g), (h), (i) are replots of the green curves from Fig. 2 (a), (b), (c).

In all subplots we show the theoretical exit rate Eq. (6) to (including) order $R^0$, evaluated on the experimental MPTs and using the diffusivity- and drift profile from Fig. 1 (b), (c). We observe that the experimental exit rate at full temporal resolution (green curves) systematically underestimates the theoretical exit rate, by an approximately time-independent value. The deviations between theoretical and experimental exit rate decrease with increasing radius, and are most prominently seen for the smallest radius $R = 0.3\,\mu$m. Indeed, in Fig. S5 (a), (d) we see that the difference between theoretical and experimental exit rate is approximately 0.5/s.

However, while for the individual exit rates in Fig. S5 (a)-(f) we observe clear deviations between theory and experiments, in the differences shown in subplots (g), (h), (i) these deviations are much smaller. This indicates that the deviations from subplots (a)-(f) dominantly depend on the radius, and only weakly on the path, and hence approximately cancel if we consider exit-rate differences.

To rationalize the deviations in the individual exit rates in Fig. S5 (a)-(f), we recall that to measure the exit rate we track whether sample trajectories remain within the tube. However, since our experimental data has a finite temporal resolution $\Delta t = 0.002\,$s, we only have information about the particle position at multiples of the timestep $\Delta t$. A trajectory can in principle leave and re-enter the tube between two observations, and our algorithm counts this as the trajectory not having left at all. This leads to a systematic underestimation of the exit rate which should become more significant as the tube radius is decreased; this is because for smaller tube radius a larger fraction of trajectories is so close to the tube boundary that the probability for exiting and re-entering the tube between to observations is non-negligible. We estimate the typical distance the colloidal particle moves between two observations as $L_{\Delta t} \equiv \sqrt{2D_{\mathrm{typ}}\Delta t} \approx 0.022\,\mu$m, where we use a typical value $D_{\mathrm{typ}} = 0.12\,(\mu\mathrm{m})^2/\mathrm{s}$ for the diffusivity (c.f. Fig. 1 (b)). For the tube radius $R = 0.3\,\mu$m we thus obtain $L_{\Delta t}/R \approx 0.073 = 7.3\%$; this means that between two observations the colloidal particle moves approximately 7.3% the tube radius. This ratio is so large that we hypothesize the finite temporal resolution of our data can affect the measured exit rate.

To provide evidence for this hypothesis, we infer the experimental exit rate again using the cloning algorithm from App. S3 for the paths $\varphi^*$, $\psi$ from Fig. 1, but at a reduced temporal resolution $5\Delta t = 0.01\,$s. We thus use the same experimental time series as before, but only consider every 5th observation to determine whether the colloidal particle has left the tube. We show the resulting exit rates and exit-rate differences in Fig. S5 as magenta curves. From subplots (a)-(f) it is apparent that at the lower temporal resolution $5\Delta t$, the estimated exit rate is systematically smaller as compared to the exit rate at full resolution $\Delta t$. Intuitively, with a lower resolution there will be more instances where trajectories exit and re-enter the tube between two observations, resulting in a smaller measured exit rate. We note that the difference between the two experimental exit rates (full temporal resolution and reduced temporal resolution) is approximately time-independent, but decreases with increasing radius. Furthermore, the finite-resolution deviations in the exit rates cancel if we consider differences; we demonstrate this in subplots (g), (h), (i), where the experimental exit-rate differences for both temporal resolutions agree.

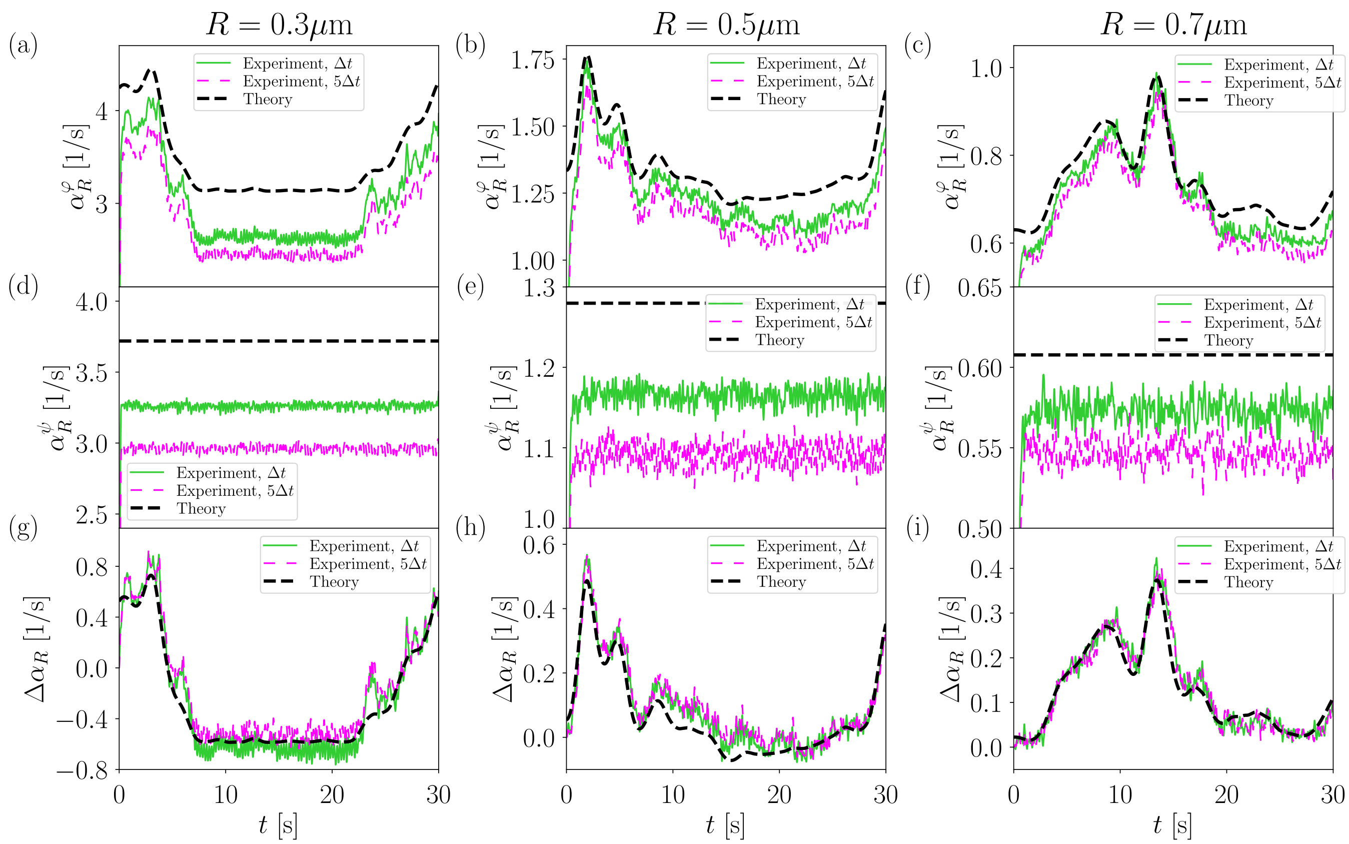


Figure S5. Subplots (a)-(f) show exit rates along the paths $\varphi^*$, $\psi$ which are depicted in Fig. 1 (f). (a)-(c) Exit rate along the path $\varphi^*$ for (a) $R = 0.3\,\mu$m, (b) $R = 0.5\,\mu$m, (c) $R = 0.7\,\mu$m. (d)-(f) Exit rate along the path $\psi$ for (d) $R = 0.3\,\mu$m, (e) $R = 0.5\,\mu$m, (f) $R = 0.7\,\mu$m. Subplots (g), (h), (i) show the exit-rate difference Eq. (4) for (g) $R = 0.3\,\mu$m, (h) $R = 0.5\,\mu$m, (i) $R = 0.7\,\mu$m. For example, each of the curves in subplot (g) is obtained as difference between the corresponding curves in (a), (d). In all subplots, the black dashed lines represent the theoretical formula Eq. (6), evaluating using the smoothed potential and diffusivity from Fig. 1 (b), (c). While the green solid lines are obtained via the algorithm described in App. S3 applied to the experimental data at full time resolution $\Delta t = 0.002\,$s, for the magenta dashed lines we use the experimental data at the lower resolution $5\Delta t = 0.01\,$s. We emphasize that for all evaluations of $\varphi^*$ for the data in this plot, we use the experimentally determined path at full resolution, shown as green solid curve in Fig. 1 (f).

Overall, the deviations in Fig. S5 between the theoretical (black) and the experimental data at full temporal resolution (green) are qualitatively similar to the deviations between the experimental data at full (green) and lower resolution (magenta). We thus conclude that the deviations between theory and full-resolution experimental results in Fig. S5 (a)-(i) are very likely due to the finite temporal resolution of our experimental time series. Since these finite-resolution effects are suppressed in exit-rate differences, we consider exit-rate differences throughout this paper.

[1] Jannes Gladrow, Ulrich F. Keyser, R. Adhikari, and Julian Kappler, "Experimental Measurement of Relative Path Probabilities and Stochastic Actions," Physical Review X **11**, 031022 (2021).

[2] Crispin W. Gardiner, Stochastic methods: a handbook for the natural and social sciences, 4th ed., Springer series in synergetics (Springer, Berlin, 2009).

[3] Julian Kappler, "Cloning algorithm for measuring rare events from stochastic time series, https://github.com/juliankappler/cloning_algorithm," ().

[4] Nikolaus Hansen, Youhei Akimoto, and Petr Baudis, "CMA-ES/pycma: r2.7.0," (2019), 10.5281/ZENODO.2559634, publisher: Zenodo.

[5] Julian Kappler, "Pytubular: Python module for the evaluation of probability densities and exit rates in the tubular ensemble, https://github.com/juliankappler/pytubular," ().

[6] Alice L. Thorneywork, Jannes Gladrow, Ulrich F. Keyser, Michael E. Cates, Ronojoy Adhikari, and Julian Kappler,

"Resolution dependence of most probable pathways with state-dependent diffusivity," .
